# Supplementary material for: Trustworthy and Efficient LLMs Meet Databases
Source: arXiv:2412.18022 source file (2024-12-23)
Supplement: Supplementary file 1 [file appendix.tex]

\vspace*{-0.2cm}
\section*{Appendix}
\vspace*{-0.15cm}
\appendix
